# Supplementary material for: Theoretical mapping of interaction between alkali metal atoms adsorbed on graphene-like BC3 monolayer
Source: arXiv:2104.02431 source file (2021-06-04)
Supplement: Supplementary file 1 [file supplem.pdf]

# Theoretical mapping of interaction between alkali metal atoms adsorbed on graphene-like $BC_3$ monolayer: **Supplementary information**

*Kazem Zhour Andrei Postnikov*

Kazem Zhour
kazem.zhour@gmail.com
Andrei Postnikov
LCP-A2MC, Université de Lorraine, 1 Bd Arago, F-57078 Metz Cedex 3, France
andrei.postnikov@univ-lorraine.fr

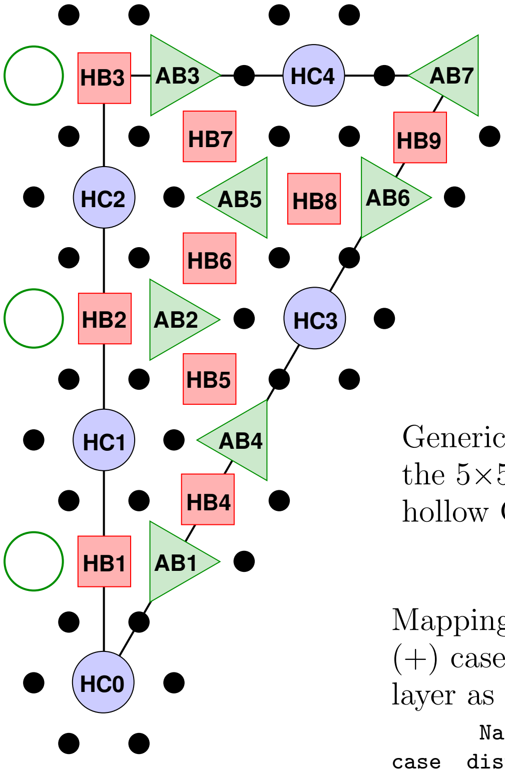


Generic labeling of adsorption sites in the irreducible wedge of the 5×5 supercell of $BC_3$. HC0 indicates the reference atom in hollow $C_6$ position.

Mapping of Na–Na interaction (Na with $2p$ in the valence). For (+) cases, the probing atom is at the same side of the $BC_3$ monolayer as the reference atom, for (−) cases – at the opposite side.

| case | Na-Na dist.(Ang) | E-E(+HC4) (eV) | case | Na-Na dist.(Ang) | E-E(-HC4) (eV) |
|---|---|---|---|---|---|
| | | | -HC0 | 0.000 | 0.183088 |
| +HC1 | 5.240 | 0.238902 | -HC1 | 5.170 | 0.005543 |
| +HC2 | 10.342 | 0.003011 | -HC2 | 10.340 | -0.010213 |
| +HC3 | 8.958 | 0.028624 | -HC3 | 8.955 | -0.002729 |
| +HC4 | 13.679 | 0.000000 | -HC4 | 13.678 | 0.0 |
| +HB1 | | | -HB1 | 2.586 | 0.054336 |
| +HB2 | 7.762 | 0.074429 | -HB2 | 7.755 | 0.013946 |
| +HB3 | 12.925 | 0.024899 | -HB3 | 12.925 | 0.019617 |
| +HB4 | 4.873 | 0.264464 | -HB4 | 4.476 | 0.002518 |
| +HB5 | 6.852 | 0.111659 | -HB5 | 6.840 | 0.018315 |
| +HB6 | 9.324 | 0.025535 | -HB6 | 9.320 | -0.001277 |
| +HB7 | 11.847 | 0.009533 | -HB7 | 11.846 | 0.004914 |
| +HB8 | 11.269 | 0.019805 | -HB8 | 11.267 | 0.019805 |
| +HB9 | 13.433 | 0.016415 | -HB9 | 13.432 | 0.018506 |
| +AB1 | 5.262 | 0.286819 | -AB1 | 2.989 | 0.132338 |
| +AB2 | | | -AB2 | 7.898 | 0.116372 |
| +AB3 | 13.011 | 0.123325 | -AB3 | 13.010 | 0.119467 |
| +AB4 | 5.985 | 0.272301 | -AB4 | 5.970 | 0.130265 |
| +AB5 | 10.763 | 0.123710 | -AB5 | 10.763 | 0.113549 |
| +AB6 | 11.940 | 0.136718 | -AB6 | 11.940 | 0.133477 |
| +AB7 | 14.925 | 0.119163 | -AB7 | 14.925 | 0.121376 |

Mapping of K–K interaction; notation is similar as for Na–Na.

| case | K-K dist.(Ang) | E-E(+HC4) (eV) |
|---|---|---|
| +HC1 | 5.783 | 0.246351 |
| +HC2 | 10.352 | 0.018047 |
| +HC3 | 8.963 | 0.047382 |
| +HC4 | 13.675 | 0.0 |
| +HB1 | 7.875 | 0.112286 |
| +HB2 | 7.830 | 0.118158 |
| +HB3 | 12.925 | 0.039876 |
| +HB4 | 6.147 | 0.306076 |
| +HB5 | 7.223 | 0.151215 |
| +HB6 | 9.348 | 0.053250 |
| +HB7 | 11.851 | 0.025300 |
| +HB8 | 11.271 | 0.040387 |
| +HB9 | 13.431 | 0.027934 |
| +AB2 | 7.929 | 0.158185 |
| +AB3 | 13.012 | 0.078152 |
| +AB4 | 7.238 | 0.211174 |
| +AB5 | 10.797 | 0.081680 |
| +AB6 | 11.922 | 0.084225 |
| +AB7 | 14.925 | 0.069158 |

| case | K-K dist.(Ang) | E-E(-HC2) (eV) |
|---|---|---|
| -HC0 | 0.0 | 0.102980 |
| -HC1 | 6.178 | 0.007865 |
| -HC2 | 10.350 | 0.0 |
| -HC3 | 8.957 | 0.001628 |
| -HC4 | 13.674 | 0.003020 |
| -HB1 | 2.581 | 0.040606 |
| -HB2 | 7.764 | 0.035710 |
| -HB3 | 12.925 | 0.037395 |
| -HB4 | 4.464 | 0.018808 |
| -HB5 | 6.840 | 0.033740 |
| -HB6 | 9.331 | 0.019335 |
| -HB7 | 11.850 | 0.021689 |
| -HB8 | 11.268 | 0.034256 |
| -HB9 | 13.430 | 0.033589 |
| -AB1 | 3.028 | 0.085426 |
| -AB2 | 7.893 | 0.074205 |
| -AB3 | 13.012 | 0.074581 |
| -AB4 | 5.965 | 0.081950 |
| -AB5 | 10.773 | 0.070414 |
| -AB6 | 11.913 | 0.080770 |
| -AB7 | 14.925 | 0.075199 |
